# Supplementary material for: A Scoping Review of Mixed Initiative Visual Analytics in the Automation Renaissance
Source: arXiv:2509.19152 source file (2026-06-09)
Supplement: Supplementary file 1 [file manuscript_revision_supplemental.tex]

% ---------------------------------------------------------------------------
% Author guideline and sample document for EG publication using LaTeX2e input
% D.Fellner, v1.21, Jan 08, 2024
\documentclass[onecolumn]{egpubl}
\usepackage{eurovis2026}

% --- for  Annual CONFERENCE
% \ConferenceSubmission   % uncomment for Conference submission
% \ConferencePaper        % uncomment for (final) Conference Paper
% \STAR                   % uncomment for STAR contribution
% \Tutorial               % uncomment for Tutorial contribution
% \ShortPresentation      % uncomment for (final) Short Conference Presentation
% \Areas                  % uncomment for Areas contribution
% \Education              % uncomment for Education contribution
% \Poster                 % uncomment for Poster contribution
% \DC                     % uncomment for Doctoral Consortium
%
% --- for  CGF Journal
% \JournalSubmission    % uncomment for submission to Computer Graphics Forum
% \JournalPaper         % uncomment for final version of Journal Paper
%
% --- for  CGF Journal: special issue
% \SpecialIssueSubmission    % uncomment for submission to , special issue
\SpecialIssuePaper         % uncomment for final version of Computer Graphics Forum, special issue
%                          % EuroVis, SGP, Rendering, PG
% --- for  EG Workshop Proceedings
% \WsSubmission      % uncomment for submission to EG Workshop
% \WsPaper           % uncomment for final version of EG Workshop contribution
% \WsSubmissionJoint % for joint events, for example ICAT-EGVE
% \WsPaperJoint      % for joint events, for example ICAT-EGVE
% \Expressive        % for SBIM, CAe, NPAR
% \DigitalHeritagePaper
% \PaperL2P          % for events EG only asks for License to Publish

% --- for EuroVis 
% for full papers use \SpecialIssuePaper
% \STAREurovis   % for EuroVis additional material 
% \EuroVisPoster % for EuroVis additional material 
% \EuroVisShort  % for EuroVis additional material
% \MedicalPrize  % uncomment for Medical Prize (Dirk Bartz) contribution, since 2021 part of EuroVis
% \EuroVisEducation              % uncomment for Education contribution

% Licences: for CGF Journal (EG conf. full papers and STARs, EuroVis conf. full papers and STARs, SR, SGP, PG)
% please choose the correct license
%\CGFStandardLicense
\CGFccby
%\CGFccbync
%\CGFccbyncnd

% !! *please* don't change anything above
% !! unless you REALLY know what you are doing
% ------------------------------------------------------------------------
\usepackage[T1]{fontenc}
\usepackage{dfadobe}  
\usepackage{pdflscape}
\usepackage[strings]{underscore}
\usepackage[normalem]{ulem}
% \usepackage{cite}  % comment out for biblatex with backend=biber
% ---------------------------
%\biberVersion
\BibtexOrBiblatex
\usepackage[backend=biber,bibstyle=EG,citestyle=alphabetic,maxcitenames=2,
  mincitenames=1]{biblatex} 
\usepackage{hyperref}
\addbibresource{manuscript.bib}
% ---------------------------  

\DeclareCiteCommand{\citet}
  {\usebibmacro{prenote}}
  {%
    \begingroup

    \printnames{labelname}%
    \endgroup
    \addspace
    \mkbibbrackets{\usebibmacro{cite}}%
  }
  {\multicitedelim}
  {\usebibmacro{postnote}}

\electronicVersion
% \PrintedOrElectronic
% for including postscript figures
% mind: package option 'draft' will replace PS figure by a filename within a frame
\ifpdf \usepackage[pdftex]{graphicx} \pdfcompresslevel=9
\else \usepackage[dvips]{graphicx} \fi

\usepackage{egweblnk}
% end of prologue

\usepackage{float}
\usepackage[skins]{tcolorbox}
\usepackage[HTML,table,xcdraw]{xcolor}
\usepackage{tabularx}
\usepackage{booktabs}
\usepackage{enumitem}
\usepackage{multicol}
\usepackage{longtable}
\usepackage{amsmath}
\setlength{\multicolsep}{0pt}
\usepackage{multirow}
\usepackage{graphicx}
\usepackage{hyperref}
\hypersetup{
        colorlinks=true,
        allcolors=black
    }
%% Included packages
\usepackage{amsmath}
\usepackage{amssymb}

%% Custom commands
% \newcommand{\acro}[1]{\textsc{\MakeLowercase{#1}}}

\definecolor{aiAgentColor}{HTML}{0092E9} % red
\definecolor{humanAgentColor}{HTML}{C96A20} % blue
\definecolor{sharedGoalsColor}{HTML}{7C546E} % purple
\definecolor{miImpactColor}{HTML}{3A8435} % green
\definecolor{miPrinciplesColor}{HTML}{C00000} % gold/yellow
% \definecolor{levelOfAutoColor}{cmyk}{0.78, 0.72, 0.67, 0.27} % dark gray
\definecolor{evaluationColor}{HTML}{156082} % dark blue

%% Custom colors
% \definecolor{motivationGreen}{cmyk}{0.70,0,1,0.28}
\definecolor{levelOfAutoColor}{HTML}{404040} % teal

\newif\ifrevisions
% \revisionstrue   % Show revisions
\revisionsfalse % Hide revisions

\ifrevisions 
     
    \long\def\deleted#1{{\color{red}\sout{#1}}} 
\else 
     
    \long\def\deleted#1{} 
\fi 

\input{manuscript_revision_supplemental_content.inc}
